# Supplementary material for: Optimization and Evaluation of Nested Queries and Procedures
Source: arXiv:0911.0508 source file (2009-11-03)
Supplement: Supplementary file 2 [file bpo_javamapping.tex]

\chapter{API and Code Patterns}
As mentioned in \refsec{sec:perf:chap:bpo}, we implemented the transformation
rules for Java because tools for Java program analysis are available 
in public domain. We make use of the {\em SOOT} optimization framework 
for obtaining data dependence information. To simplify the task of 
recognizing query execution statements and code patterns that match
a rule, our current implementation requires that queries and updates 
be performed using our API layer built on top of JDBC. During rewrite,
we recognize these calls and transform them for batched bindings when 
possible. In this section, we give the details of our API layer and
the Java code patterns, which map to constructs described earlier,
in this thesis.
{\em SOOT} uses an intermediate code representation called {\em Jimple}. 
Our implementation works on {\em Jimple} and transforms it back to Java. 
Recognizing {\em Jimple} code patterns corresponding to each of our 
API calls and Java code patters is relatively straight forward and 
we omit the details.

\eat{
This mapping, used in our implementation, employs a custom API layer 
built on top of JDBC and is designed for easy recognition of program 
fragments that match the rule antecedents. It is possible to define 
alternative mappings - {\em e.g.}, a mapping that helps rewrite programs 
that directly make use of JDBC API. Mappings to languages like PL/SQL or
TSQL are more direct as the language constructs used in this thesis are
similar to the ones in those languages ({\em e.g.}, cursor loops).
}

\begin{itemize}
\item{\bf Query/Update Execution Statements}:
The class {\em DBI} in our implementation provides various methods for 
executing queries and updates.

{\small
\begin{itemize}
\item {\em Record executeScalarQuery(int queryId, Record params)}
%\item {\em Record executeScalarQuery(int queryId, \\ \hspace*{37mm} Record params)}
\item {\em Table executeQuery(int queryId, Record params)}
\item {\em int executeUpdate(int queryId, Record params)}
\end{itemize}
}

The {\em queryId} specifies a parameterized SQL query or update 
statement in a query registry. Unlike JDBC, where the query string 
is directly specified in the program, we make use of a registry.
The query registry, in addition to the query string, also contains 
the manually written batched form for the query.
Unlike position-based parameters 
in JDBC, we use named parameters. The {\em Record} class is used
to pass parameters as name-value pairs and also to obtain the
result of a scalar query. The class {\em Table} implements a 
tuple set and is used to retrieve query results, and for constructing
parameter batches.
% Sample entries in the registry
%SELECT city, state, zip FROM contactinfo WHERE emp-id=[empid]
%SELECT empid, city, state, zip FROM [batchtable] b, contactinfo c WHERE c.emp-id=b.empid

\begin{figure}[ht]
\begin{center}
\begin{tabular}{lcl}
\begin{minipage}{0.6\textwidth}
\scriptsize{
\ordinalg{
\\
%{\bf In Java} \\
Table res = DBI.executeQuery($\ldots$); \\
Iterator resIter = res.iterator(); \\
xxx\=xxx\=xxx\=\kill
while(resIter.hasNext()) $\{$ \\
    \> Record r = (Record) resIter.next(); \\
    \> $\ldots$ \\
$\}$ \\
}
}
\end{minipage}
&
\begin{minipage}{0.1\textwidth}
$\Longrightarrow$ \\
\end{minipage}
&
\begin{minipage}{0.3\textwidth}
\scriptsize{
\ordinalg{
%\noindent {\bf A Cursor Loop} \\
for each r in {\em query} \\
\> $\ldots$ \\
end loop; 
}
}
\end{minipage}
\end{tabular}
\end{center}
\caption{Pattern for Cursor Loops}
\label{fig:cursorloop}
\end{figure}

\item{\bf Looping Statements}:
{\em while} loops have a direct mapping to Java. Unlike some of
the procedural languages offered by database systems (e.g., PL/SQL), 
Java does not have cursor loops. Each cursor loop maps to a sequence 
of statements in Java. \reffig{fig:cursorloop} shows the code pattern.

\item{\bf Batched Execution}:
The class {\em Table} in our implemen\-tation can be used for constructing 
parameter batches row by row using the method {\em addRecord(Record r)}. The
DBI class has methods for executing batched forms of queries by passing
a batch of parameters and also for merging back the results. These methods 
are used by the transformed program (generated code).

{\small
\begin{itemize}
%\item {\em Table executeBatchedQuery(int queryId, \\ \hspace*{8mm}Table paramBatch)}
\item {\em Table executeBatchedQuery(int queryId, Table paramBatch, FilterPred pred)}
%\item {\em void executeBatchedUpdate(int queryId, \\ \hspace*{8mm}Table paramBatch)}
\item {\em void executeBatchedUpdate(int queryId, Table paramBatch, FilterPred pred)}
\end{itemize}
}

\item{\bf Other Constructs}:
Control flow, assignment and \- other constructs in the simple procedural
language used in this thesis have a direct mapping to Java. Conditional
statements, generated when control-dependencies are converted to
flow-dependencies, are Java {\em if} statements, where the {\em if-block}
contains a single statement and the predicate is a boolean variable.

\end{itemize}
