# Supplementary material for: Optimization and Evaluation of Nested Queries and Procedures
Source: arXiv:0911.0508 source file (2009-11-03)
Supplement: Supplementary file 4 [file bpo_queries.tex]

%\chapter{Procedures used in Experiments}
\chapter{Procedures Used in Experiments}
\label{appendix1}
%\section*{Procedure for Experiment 2}
This section gives pseudocode for the additional procedures used for
performance evaluation in \refsec{sec:perf:chap:bpo}. \reffig{fig:nicproc}
shows the procedure for Experiment-3 and the procedure for Experiment-2 is
given in \reffig{fig:proc2}. The functionality implemented by these
procedures was explained earlier, in \refsec{sec:perf:chap:bpo}.

%\section*{Value Range Expansion: Exp 3}
\begin{figure}[ht]
\begin{minipage}{1.0\textwidth}
\scriptsize{
\ordinalg{
PROCEDURE expand-issued-forms(DATE issuedate) \\
DECLARE \\
    \> INT num; \\
BEGIN \\
    \> FOR EACH irec IN SELECT agent$\_$id, start$\_$no, end$\_$no, issue$\_$date \\
    \> \> \> \> \> FROM issued$\_$forms WHERE issue$\_$date = issuedate LOOP \\
    \> \> num := irec.start$\_$no; \\
    \> \> WHILE (num $<=$ irec.end$\_$no) LOOP \\
    \> \> \> INSERT INTO forms-master VALUES (num, irec.agent$\_$id, irec.issue$\_$date, 'NEW'); \\
    \> \> \> num := num + 1; \\
    \> \> END LOOP; \\
    \> END LOOP; \\
END; \\
}
}
\end{minipage}
\caption{Procedure for Experiment 3}
\label{fig:nicproc}
\end{figure}

\begin{figure}[ht]
\begin{minipage}{1.0\textwidth}
\scriptsize{
\ordinalg{
PROCEDURE emp-upload(VARCHAR filename) \\
DECLARE \\
    \> // Data types of local variables omitted for brevity. \\
    \> empid, clientid, iempid, optcode, optinfo, termcode, taxinfo, \\
    \> city, state, zip, operation, curtaxinfo, curcity, curstate, curzip\\
BEGIN \\
\>    fd := open(filename); \\
\>    linestr := readline(fd); \\
\>    WHILE (linestr $!=$ null) LOOP \\
\>  \>  tokenize linestr and extract empid, clientid, optcode, $\ldots$ zip \\
\>  \>  // some validation and pre-processing code  \\
\>  \>  if(optcode == 0) \\
\>  \>   \> optinfo = ... ; \\
\> \>  $\ldots$ \\
\\
\> \>   SELECT internl-empid into iempid, tax-info into curtaxinfo, \\
\> \>   FROM options WHERE client-id=clientid AND emp-id=empid; \\
\\
\> \>   // If options has no record for the employee \\
\> \>   if(iempid == null) $\{$ \\ 
\> \> \>    operation := 1;  // we must insert \\
\> \> \>    iempid := gen-new-id(); \\
\> \>   $\}$ \\
\> \>   else $\{$ \\
\> \> \>    operation := 2;  // we must update \\
\\
\> \> \>    SELECT city into curcity, state into curstate, zip into curzip \\
\> \> \>    FROM contactinfo  WHERE internal-empid=iempid; \\
\\      
\> \> \>    // Retain the current values if new ones are blank \\
\> \> \>    if(taxinfo == $""$) \\
\>  \> \>  \>   taxinfo := curtaxinfo; \\
\> \> \>    if(city == $""$) \\
\> \> \> \>     city := curcity; \\
\> \> \>    $\ldots$ \\
\> \> \>    $\ldots$ \\
\eat{
\> \> \>    if(state == "") \\
\> \> \> \>     state := curstate; \\
\> \> \>   if(zip  == "") \\
\> \> \> \>    zip := curzip; \\
}
\> \> $\}$ \\
\> \>  if(operation == 1) $\{$ \\
\> \> \>  INSERT INTO options VALUES (iempid, clientid, ... optinfo, ... taxinfo); \\
\> \> \>  INSERT INTO contactinfo VALUES(iempid, city, state, zip); \\
\> \>  $\}$ \\
\> \>   else $\{$ \\
\> \> \>    UPDATE options set option-info=optinfo, $\ldots$ tax-info=taxinfo \\
\> \> \>    WHERE internal-empid=iempid; \\
\> \> \>    UPDATE contactinfo SET city=city, state=state, zip=zip \\
\> \> \>    WHERE internal-empid=iempid; \\
\> \>  $\}$ \\
\> \>   linestr := readline(fd); \\
\>  END LOOP; \\
END; \\
}
}
\end{minipage}
\caption{Procedure for Experiment 2}
\label{fig:proc2}
\end{figure}
