# Supplementary material for: Optimization and Evaluation of Nested Queries and Procedures
Source: arXiv:0911.0508 source file (2009-11-03)
Supplement: Supplementary file 7 [file extra-rules.tex]

\subsection*{Extra Rules}
\label{extra-rules}
%This appendix provides few additional transformation rules.
Rule 7 in \reffig{fig:rule-arith} and Rule 8 in \reffig{fig:rule-inline} are
useful in replacing loops containing simple expressions and assignment with
relational operators and avoiding materialization of intermediate results.
As mentioned in \refchap{chap:concl} these rules can be used to
build a single dataflow for queries, which invoke UDFs that run inside the
database.  The {\em trivial batched form} (see
\reffig{fig:trivial-batched-form}) constructs the {\em return table}
iteratively.  Rule 9 in \reffig{fig:rule-return} is useful to convert this
into a set valued expression. The example in Appendix
\ref{step-by-step-trans} illustrates the use of this rule.

\begin{figure}[ht]
\begin{minipage}{0.5\textwidth}
{\bf Rule 7}
{\scriptsize
\begin{transrule}
FOR EACH t BY REF IN r [ORDER BY key] LOOP \\
\>    t.b = {\em arith-expr}$(t.a_1, t.a_2, \ldots t.a_n)$;  \\
END LOOP; \\
\hspace{10mm} {\large $\Updownarrow$}
\end{transrule}
}
\vspace{-15pt}
{\small
\begin{transrule}
%$r = \Pi_{\{r.*-b\}, \textit{arith-expr}(t.a_1, t.a_2, \ldots t.a_n)\ as\ b}(r)$ 
$r = \Pi_{A, \textit{arith-expr}(t.a_1, t.a_2, \ldots t.a_n)\ as\ b}(r)$, 
\\
where {\em A=schema(r)}$-$$\{b\}$
\end{transrule}
}
\end{minipage}
\caption{Loops with Arithmetic Expressions and Assignment}
\label{fig:rule-arith}
\end{figure}

\begin{figure}[ht]
\begin{minipage}{0.5\textwidth}
{\bf Rule 8}
{\scriptsize
\begin{transrule}
{\small Let expr1 be a side-effect free expression ({\em e.g.,} a query).} \\
\\
TABLE r1 = expr1(); \\
TABLE r2 = expr2(r1);
%\ \ \ {\large $\Leftrightarrow$}\ \ \  TABLE r2 = expr2(expr1); \\
{\em dead}(r1)  // r1 unused hereafter \\
\hspace{10mm} {\large $\Updownarrow$} \\
TABLE r2 = expr2(expr1);
\end{transrule}
}
\end{minipage}
\caption{Rule for Avoiding Materialization}
\label{fig:rule-inline}
\end{figure}

\begin{figure}[ht]
\begin{minipage}{0.5\textwidth}
{\bf Rule 9}
\scriptsize{
\begin{transrule}
TABLE result; \\
FOR EACH t [BY REF] IN r [ORDER BY key] LOOP \\
%\>    result.addRecord($(t.a_1, t.a_2, \ldots t.a_n)$);  \\
\>    result.addRecord($(c_1, c_2, \ldots c_n)$);  \\
\>    // where each $c_i$ is a function of attributes of {\em t}. \\
END LOOP; \\
RETURN result;\\
\hspace{10mm} {\large $\Updownarrow$} \\
RETURN SELECT $c_1, c_2, \ldots c_n$ FROM r;
\end{transrule}
}
\end{minipage}
\caption{Rule for {\small RETURN} Statement}
\label{fig:rule-return}
\end{figure}
